# Supplementary material for: sGDML: Constructing Accurate and Data Efficient Molecular Force Fields Using Machine Learning
Source: arXiv:1812.04986 ancillary file (2019-03-02)
Supplement: Supplementary file 1 [file supplement.pdf]

# sGDML: Constructing Accurate and Data Efficient Molecular Force Fields Using Machine Learning
Supplementary Information

Stefan Chmiela,[1] Huziel E. Sauceda,[2] Igor Poltavsky,[3] Klaus-Robert Müller,[1,4,5,*] and Alexandre Tkatchenko[3,†]

[1]*Machine Learning Group, Technische Universität Berlin, 10587 Berlin, Germany*
[2]*Fritz-Haber-Institut der Max-Planck-Gesellschaft, 14195 Berlin, Germany*
[3]*Physics and Materials Science Research Unit, University of Luxembourg, L-1511 Luxembourg, Luxembourg*
[4]*Department of Brain and Cognitive Engineering, Korea University, Anam-dong, Seongbuk-gu, Seoul 136-713, Korea*
[5]*Max Planck Institute for Informatics, Stuhlsatzenhausweg, 66123 Saarbrücken, Germany*

## S1. GDML DERIVATION

When training a GDML model [1], the following quadratic objective function over $M$ training points is minimized:

$$\mathcal{L}(\mathbf{\Omega}) = \sum_i^M (\mathbf{J}_{\Phi_i}\vec{\omega}_i - \mathbf{F}_i)^2 + \lambda\|\mathbf{\Omega}\|^2 \tag{1}$$

Here, $\mathbf{J}_{\Phi_i} = \mathbf{J}_{\Phi(\vec{x}_i)}$ are the $3N \times F$ Jacobi matrices of a non-linear feature transform of the training geometries $\vec{x}_i$ into $F$-dimensional space, weighted by parameter vectors $\vec{\omega}_i$. $\mathbf{F}_i$ contains the atomic forces (e.g. negative energy gradients) corresponding to each geometry, stacked into a vector. For the sake of simplicity we will assume that the geometry encoded in $\vec{x}_i$ is simply represented in Cartesian coordinates, but we will introduce a descriptor in the final formulation of the model. In addition, the norm of the coefficients $\mathbf{\Omega} = [\vec{\omega}_1^\top, \ldots, \vec{\omega}_M^\top]^\top$ is penalized as way to regularize the complexity of the solution. The regularization strength is tuned via a hyper-parameter $\lambda$.

To find the minimum, we set the derivative of this cost function to zero:

$$\frac{\partial\mathcal{L}}{\partial\mathbf{\Omega}} = 2\sum_i^M \mathbf{J}_{\Phi_i}^\top(\mathbf{J}_{\Phi_i}\vec{\omega}_i - \mathbf{F}_i) + 2\lambda\mathbf{\Omega} = \vec{0} \tag{2}$$

giving

$$\begin{aligned} \sum_i^M \mathbf{J}_{\Phi_i}^\top\mathbf{J}_{\Phi_i}\vec{\omega}_i - \mathbf{J}_{\Phi_i}^\top\mathbf{F}_i &= \lambda\mathbf{\Omega} \\ \rightarrow \mathbf{\Omega} &= \left(\lambda\mathbb{I}_F + \sum_i^M \mathbf{J}_{\Phi_i}^\top\mathbf{J}_{\Phi_i}\right)^{-1}\sum_j^M \mathbf{J}_{\Phi_j}^\top\mathbf{F}_j \end{aligned} \tag{3}$$

We will now aggregate the Jacobi matrices for all training points into a large matrix $\mathbf{J_\Phi} = [\mathbf{J}_{\Phi_1}, \ldots, \mathbf{J}_{\Phi_M}]$ of dimension $3NM \times F$ and use pure matrix notation. We continue by applying the Woodbury matrix identity:

$$\begin{aligned} \mathbf{\Omega} &= (\mathbf{J_\Phi}^\top\mathbf{J_\Phi} + \lambda\mathbb{I}_F)^{-1}\mathbf{J_\Phi}^\top\mathbf{F} \\ &= \mathbf{J_\Phi}^\top\underbrace{((\mathbf{J_\Phi}\mathbf{J_\Phi}^\top + \lambda\mathbb{I}_{3NM})^{-1}\mathbf{F})}_{\mathbf{A}} \end{aligned} \tag{4}$$

This way we can solve the linear system above in $3NM \ll F$. Forces for new inputs are then computed by evaluating $\mathbf{F}_{\text{new}} = \mathbf{J}_{\Phi_{\text{new}}}\mathbf{\Omega}$, which can also be written as

$$\mathbf{F}_{\text{new}} = \mathbf{J}_{\Phi_{\text{new}}}\mathbf{J_\Phi}^\top\mathbf{A}. \tag{5}$$

* klaus-robert.mueller@tu-berlin.de
† alexandre.tkatchenko@uni.lu

This is helpful because $\mathbf{J_\Phi J_\Phi^\top}$ and $\mathbf{J}_{\Phi_\text{new}}\mathbf{J_\Phi^\top}$ are (co)variances between derivative observation in feature space and we can apply the "kernel trick" to express them via a kernel function that foregoes an explicit mapping [2]. We write the Jacobian $\mathbf{J_\Phi} = \nabla\mathbf{\Phi}^\top$ as the outer product of feature transform and derivative operator and then

$$\begin{aligned}\mathbf{J_\Phi J_\Phi^\top} &= \nabla\mathbf{\Phi}^\top(\nabla\mathbf{\Phi}^\top)^\top \\ &= \nabla\underbrace{\mathbf{\Phi}^\top\mathbf{\Phi}}_{\kappa}\nabla^\top\end{aligned} \tag{6}$$

to substitute the inner product of feature transformations with a scalar-valued kernel function. The force field kernel in GDML is thus a matrix with entries $(\kappa)_{ij} = {}^{\partial^2\kappa}/_{\partial\vec{x}_i\partial\vec{x}'_j}$. It is equivalent (up to sign) to the Hessian of the original scalar-valued kernel function with respect to either one of both inputs, if $\kappa$ is stationary, i.e. $\kappa(\vec{x},\vec{x}') = \tilde{\kappa}(\vec{x}-\vec{x}')$. With $\tau = \vec{x}-\vec{x}'$, the second derivative is

$$\frac{\partial^2\tilde{\kappa}}{\partial\vec{x}\partial\vec{x}'} = \frac{\partial^2\tilde{\kappa}}{\partial\tau^2}\frac{\partial\tau}{\partial\vec{x}}\frac{\partial\tau}{\partial\vec{x}'} = -\frac{\partial^2\tilde{\kappa}}{\partial\tau^2}\left(\frac{\partial\tau}{\partial\vec{x}}\right)^2 = \frac{\partial^2\tilde{\kappa}}{\partial^2\vec{x}}. \tag{7}$$

Finally, we rewrite Eq. 5 in a more verbose way and obtain with $\mathbf{A} = [\vec{\alpha}_1^\top,\dots,\vec{\alpha}_M^\top]^\top$

$$\hat{\mathbf{f}}_\mathbf{F}(\vec{x}) = \sum_i^M\sum_j^{3N}(\vec{\alpha}_i)_j\frac{\partial}{\partial x_j}\nabla_{\vec{x}}\kappa(\vec{x},\vec{x}_i) \tag{8}$$

for the force field model, where ${}^\partial/_{\partial x_j}$ is the partial derivative with respect to the $j$-th component of the input vector. The corresponding reconstruction of the potential energy surface is recovered up to a constant via integration:

$$\hat{f}_E(\vec{x}) = \sum_i^M\sum_j^{3N}(\vec{\alpha}_i)_j\frac{\partial}{\partial x_j}\kappa(\vec{x},\vec{x}_i) + c. \tag{9}$$

Due to linearity of integration, the expression for the energy predictor $\hat{f}_E(\vec{x})$ is identical up to the second derivative operator acting on the kernel function. The inverted sign of the energy is accounted for by use of the Hessian in Eq. 8.

### A. Integration Constant

The sum of squared deviations between predicted and reference energy at every training point is minimized to estimate the integration constant. We minimize the loss function

$$\begin{aligned}\mathcal{L}(c) &= \sum_i^M(\int\hat{\mathbf{f}}_\mathbf{F}(\vec{x}_i)\,\mathrm{d}x - e_i)^2 \\ &= \sum_i^M(-\hat{f}_E(\vec{x}_i) + c - e_i)^2,\end{aligned} \tag{10}$$

which unsurprisingly gives the mean of energy deviations at every training point

$$\begin{aligned}\frac{\partial\mathcal{L}}{\partial c} &= 2\sum_i^M c - (e_i + \hat{f}_E(\vec{x}_i)) = 0 \\ &= 2Mc - 2\sum_i^M e_i + \hat{f}_E(\vec{x}_i) \\ \rightarrow c &= \frac{\sum_i^M e_i + \hat{f}_E(\vec{x}_i)}{M}\end{aligned} \tag{11}$$

as the best estimate for the integration constant.

## S2. SGDML DERIVATION

Building on GDML, sGDML is an extension that automatically recovers the relevant rigid space group and fluxional symmetries from the training dataset of molecular geometries and exercises them within the kernel function. This new symmetric kernel function then acts as a drop-in replacement for the kernel function in GDML (see Chmiela et al. [3] for details)

$$\mathrm{Hess}(\kappa_{\mathrm{sym}})(\vec{x},\vec{x}') = \frac{1}{S}\sum_{pq}^{S} \mathbf{P}_p^\top \mathrm{Hess}(\kappa)(\mathbf{P}_p\vec{x},\mathbf{P}_q\vec{x}')\mathbf{P}_q \tag{12}$$

where the $S$ symmetries are expressed as permutation matrices $\mathbf{P}$ that act on the atoms of a molecule.

## S3. DESCRIPTOR

So far, we did not include the descriptor in any of our derivations. It enters the kernel function with $\vec{x} = D(\vec{r})$ where $\vec{r}$ is the Cartesian molecular geometry. Of course, we are then interested in the Hessian w.r.t. $\vec{r}$, not $D(\vec{r})$ and hence apply the chain rule to obtain

$$\mathrm{Hess}(\kappa)_{\mathbf{D}} = \mathbf{J}_{\mathbf{D}}\,\mathrm{Hess}(\kappa)\,\mathbf{J}_{\mathbf{D}'}, \tag{13}$$

or for the force field kernel in sGDML using $\mathbf{D}(\mathbf{P}_i\vec{r}) = \mathbf{D}_{\mathbf{P}_i}$:

$$\mathrm{Hess}(\kappa_{\mathrm{sym}})_{\mathbf{D}} = \frac{1}{S}\sum_{pq}^{S} (\mathbf{J}_{\mathbf{D}_{\mathbf{P}_p}}\mathbf{P}_p)^\top \mathrm{Hess}(\kappa)(\mathbf{D}_{\mathbf{P}_p},\mathbf{D}'_{\mathbf{P}_q})\mathbf{J}_{\mathbf{D}'_{\mathbf{P}_q}}\mathbf{P}_q \tag{14}$$

See section S4 A for a concrete example using the inverse pairwise distance descriptor used in GDML and sGDML.

## S4. MATÉRN FORCE FIELD KERNEL

Here, we compute the Hessian of the (isotropic) kernel function from the parametric Matérn family,

$$\begin{aligned} \kappa : C_{v=n+\frac{1}{2}}(d) &= B(d)P_n(d), \\ B(d) &= \exp\left(-\frac{\sqrt{2v}d}{\sigma}\right), \\ P_n(d) &= \sum_{k=0}^{n}\frac{(n+k)!}{(2n)!}\binom{n}{k}\left(\frac{2\sqrt{2v}d}{\sigma}\right)^{n-k} \end{aligned} \tag{15}$$

to obtain the force field kernel as it is used in GDML and sGDML (see section S1). In this formulation, $d = \|\vec{x}-\vec{x}'\|$ is the Euclidean distance between two inputs and $\sigma$ is the length scale. It can be regarded as a generalization of the universal squared exponential kernel with variable differentiability $n$. In our application, we use $n = 2$ which yields a kernel function that is similar to the exponential kernel, but twice differentiable. Nevertheless, we derive the Hessian in full generality here. For notational convenience we write this kernel function as a product of an exponential term $B(d)$ and a polynomial $P_n(d)$ of order $n$. Then the partial derivatives in the gradient take the form

$$\frac{\partial\kappa}{\partial x_i} = B\frac{\partial P_n}{\partial x_i} + \frac{\partial B}{\partial x_i}P_n. \tag{16}$$

They are composed of the first derivatives of the polynomial

$$\frac{\partial P_n}{\partial x_i} = \sum_{k=0}^{n}\frac{(n+k)!}{(2n)!}\binom{n}{k}\frac{(n-k)(x_i-x_i')}{d^2}\left(\frac{2^{\sqrt{2}}\sqrt{v}d}{\sigma}\right)^{n-k} \tag{17}$$

and the first derivative of the exponential function

$$\frac{\partial B}{\partial x_i} = -\frac{\sqrt{2v}(x_i-x_i')}{\sigma d}\exp\left(-\frac{\sqrt{2v}d}{\sigma}\right). \tag{18}$$

Analogously, the entries in the corresponding Hessian evaluate to

$$\frac{\partial^2 \kappa}{\partial x_i \partial x_j} = B\frac{\partial^2 P_n}{\partial x_i \partial x_j} + \frac{\partial B}{\partial x_i}\frac{\partial P_n}{\partial x_j} + \frac{\partial B}{\partial x_j}\frac{\partial P_n}{\partial x_i} + \frac{\partial^2 B}{\partial x_i \partial x_j}P_n \tag{19}$$

using the second derivative of the polynomial

$$\begin{aligned}
\left[\frac{\partial^2 P_n}{\partial x_i \partial x_j}\right]_{i\neq j} &= \sum_{k=0}^{n} \frac{(n+k)!}{(2n)!}\binom{n}{k}\frac{(n-k-2)(n-k)(x_i - x_i')(x_j - x_j')}{d^4}\left(\frac{2^{\sqrt{2}}\sqrt{v}d}{\sigma}\right)^{n-k} \\
\left[\frac{\partial^2 P_n}{\partial x_i \partial x_j}\right]_{i=j} &= \left[\frac{\partial^2 P_n}{\partial x_i \partial x_j}\right]_{i\neq j} + \sum_{k=0}^{n} \frac{(n+k)!}{(2n)!}\binom{n}{k}\frac{(n-k)}{d^2}\left(\frac{2\sqrt{2v}d}{\sigma}\right)^{n-k}
\end{aligned} \tag{20}$$

and the second derivative of the exponential

$$\begin{aligned}
\left[\frac{\partial^2 B}{\partial x_i \partial x_j}\right]_{i\neq j} &= \frac{\sqrt{2v}(x_i - x_i')(x_j - x_j')(\sqrt{2v}d + \sigma)}{\sigma^2 d^3}\exp\left(-\frac{\sqrt{2v}d}{\sigma}\right) \\
\left[\frac{\partial^2 B}{\partial x_i \partial x_j}\right]_{i=j} &= \left[\frac{\partial^2 B}{\partial x_i \partial x_j}\right]_{i\neq j} + \frac{\sqrt{2v}}{\sigma d}\exp\left(-\frac{\sqrt{2v}d}{\sigma}\right).
\end{aligned} \tag{21}$$

The matrix-valued force field kernel function Hess($\kappa$) is then assembled according to Eq. 19.

### A. Pairwise Inverse Distance Descriptor

In GDML and sGMDL, we use matrices of pairwise inverse distances between atoms

$$(\mathbf{D})_{ij} = \begin{cases} \|r_i - r_j\|^{-1} & \text{for } i > j \\ 0 & \text{for } i \leq j \end{cases} \tag{22}$$

to describe molecular graphs in a translationally and rotationally invariant way. The Jacobian $\mathbf{J_D} = [\text{vec}(\nabla_{r_1}\mathbf{D}), \dots, \text{vec}(\nabla_{r_N}\mathbf{D})]^\top$ (as used in section S3) is composed of the vectorized descriptor derivatives w.r.t. to each atomic position $\vec{r}$ in Cartesian coordinates:

$$(\nabla_{r_i}\mathbf{D})_{ij/ji} = \begin{cases} (r_i - r_j)\|r_i - r_j\|^{-3} & \text{for } i > j \\ 0 & \text{for } i \leq j \end{cases}. \tag{23}$$

## S5. MEMORY REQUIREMENT FOR TRAINING

In this implementation, we train the sGDML analytically, i.e. by solving a linear system in closed form. While this approach is faster and more accurate than numerical methods (i.e. gradient descent), it is also highly memory demanding. Analytic solvers require the complete kernel matrix to be kept in memory at once. With $(M \times 3N)^2$ double precision (8 byte) entries, it dominates the memory footprint of the training process. Those numbers can be used as a rough guideline for choosing a suitable hardware platform.

## S6. TRAINING VIA THE PYTHON API

This minimal example shows how to train one individual sGDML model (without cross-validation or testing) for a particular choice of hyper-parameters $\sigma = 10$ and $\lambda = 1\text{e}{-15}$ via the Python API:

```
import sys
import numpy as np
from sgdml.train import GDMLTrain

n_train = 500
train_dataset = np.load(<train_dataset_path>)

n_train = 1000
test_dataset = np.load(<test_dataset_path>)

gdml = GDMLTrain(model)

task = gdml.create_task(train_dataset, n_train,\
                        test_dataset, n_test,\
                        sig=10, lam=1e-15)

try:
  model = gdml.train(task)
except Exception, err:
  sys.exit(err)
else:
  np.savez_compressed("model.npz", **model)
```

A comprehensive documentation is available at *http://sgdml.org/doc/*.

## S7. INTERFACES

### A. sGDML to ASE interface

The Atomic Simulation Environment (ASE) [4] is a collection of Python tools for atomistic simulations, including classical MD, structure optimization, nudged elastic band calculations and more. External force fields, like sGDML can easily be integrated as `Calculator` objects. To use the included `SGDMLCalculator`, simply import it from the sGDML package and initialize it with the path to a model file:

```
from sgdml.intf.ase import SGDMLCalculator
sgdml = SGDMLCalculator(m_paracetamol.npz)
```

Then, attach it to any `Atoms`-object:

```
mol = read_xyz(paracetamol.xyz).next()
mol.set_calculator(sgdml)
```

Please keep in mind, that the sGDML model must match the molecular geometry represented by the `Atoms`-object.

### B. sGDML to i-PI interface

The i-PI software offers an efficient and user-friendly PIMD implementation including state-of-the-art integrators and thermostats [5]. We provide the necessary interface code to use sGDML models within i-PI via a `ForceField` object that forwards forces and energies to the main simulation engine. This integration requires editing the `forcefields.py` file (in `ipi/engine/`), to which a new interface class `FFsGDML` needs to be added. Additionally, `FFsGDML` must to be declared as a new input option by updating the files `ipi/inputs/forcefields.py` and `ipi/inputs/simulation.py` accordingly. We offer patched versions of those files (compatible with i-PI 2.0) as drop-in replacements:

```
ipi_engine_forcefields.py
ipi_inputs_forcefields.py
ipi_inputs_simulation.py
```

Finally, the sGDML `ForceField` can be specified in the i-PI `input.xml`. The relevant entries are:

```
<ffsgdml name="sgdml">
</ffsgdml>
<system>
...
  <forces>
    <force forcefield="sgdml"> </force>
    sGDMLmodel="sGDML_model_name.npz"
  </forces>
...
</system>
```

where `sGDMLmodel` is the name of the appropriate model file.

### 1. *Example: Paracetamol MD*

To verify the correct installation of the i-PI interface, we include an ready-to-run example consisting of the following input files:

```
input.xml
paracetamol_input_geometry.xyz
m_paracetamol.npz
```

The MD simulation is started with

```
$ python i-pi input.xml
```

This example takes a couple of minutes to finish on a regular laptop computer. The resulting trajectory will be stored in `paracetamol_pos_0.xyz` and can be easily visualized, e.g. using Jmol.


[1] S. Chmiela, A. Tkatchenko, H. E. Sauceda, I. Poltavsky, K. T. Schütt, and K.-R. Müller, Sci. Adv. **3**, e1603015 (2017).

[2] K.-R. Müller, S. Mika, G. Rätsch, K. Tsuda, and B. Schölkopf, IEEE Trans. Neural Netw. Learn. Syst. **12**, 181 (2001).

[3] S. Chmiela, H. E. Sauceda, K.-R. Müller, and A. Tkatchenko, Nat. Commun. **9**, 3887 (2018).

[4] A. H. Larsen, J. J. Mortensen, J. Blomqvist, I. E. Castelli, R. Christensen, M. Duak, J. Friis, M. N. Groves, B. Hammer, C. Hargus, E. D. Hermes, P. C. Jennings, P. B. Jensen, J. Kermode, J. R. Kitchin, E. L. Kolsbjerg, J. Kubal, K. Kaasbjerg, S. Lysgaard, J. B. Maronsson, T. Maxson, T. Olsen, L. Pastewka, A. Peterson, C. Rostgaard, J. Schitz, O. Schtt, M. Strange, K. S. Thygesen, T. Vegge, L. Vilhelmsen, M. Walter, Z. Zeng, and K. W. Jacobsen, J. Phys. Condens. Matter **29**, 273002 (2017).

[5] V. Kapil, M. Rossi, O. Marsalek, R. Petraglia, Y. Litman, T. Spura, B. Cheng, A. Cuzzocrea, R. H. Meiner, D. M. Wilkins, P. Juda, S. P. Bienvenue, W. Fang, J. Kessler, I. Poltavsky, S. Vandenbrande, J. Wieme, C. Corminboeuf, T. D. Kühne, D. E. Manolopoulos, T. E. Markland, J. O. Richardson, A. Tkatchenko, G. A. Tribello, V. V. Speybroeck, and M. Ceriotti, Comput. Phys. Commun. (2018).
